# Supplementary material for: Receiver Functions in the San Fernando Valley, California: Graph-Regularized Bayesian Approach for Gravity-Informed Mapping
Source: arXiv:2601.02575 source file (2026-01-05)
Supplement: Supplementary file 1 [file SuppInfo_SFV_compressed.pdf]

*JGR: Solid Earth*

Supporting Information for

# Receiver Functions in the San Fernando Valley, California: Graph-Regularized Bayesian Approach for Gravity-Informed Mapping

Valeria Villa[1], Robert W. Clayton[1], Patricia Persaud[2]

[1]Seismolab, California Institute of Technology, Pasadena, California, USA

[2]Department of Geosciences, University of Arizona, Tucson, Arizona, U.S.A

## Contents of this file

Figures S1 to S11
Tables S1

## Introduction

The following are additional plots that support the techniques and models described in the main text. All captions and text within the figures fully describe the message conveyed by each figure or mentioned in the main text.

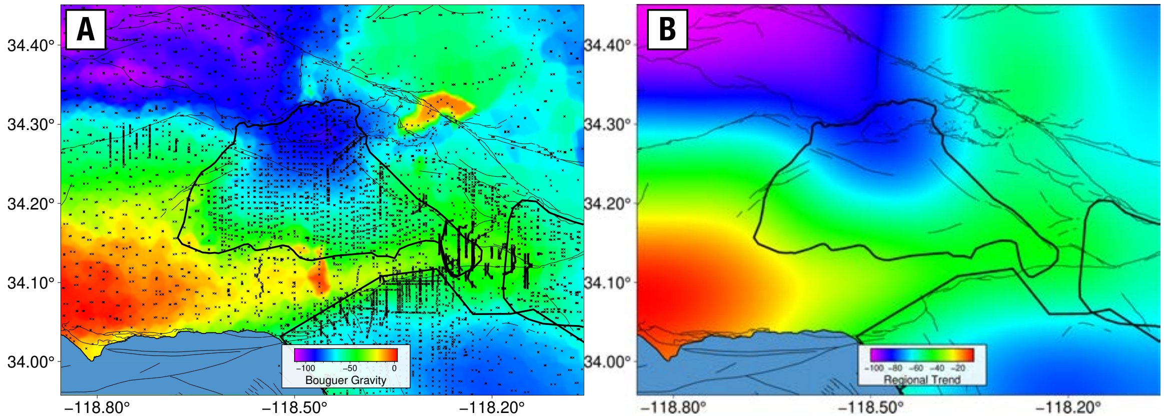


**Figure S1.** A) Regional Bouguer gravity in the San Fernando Valley and surrounding areas. The crosses show to the gravity stations (Clayton, 2022). B) Regional trend using a 5-km 2D Gaussian filter.

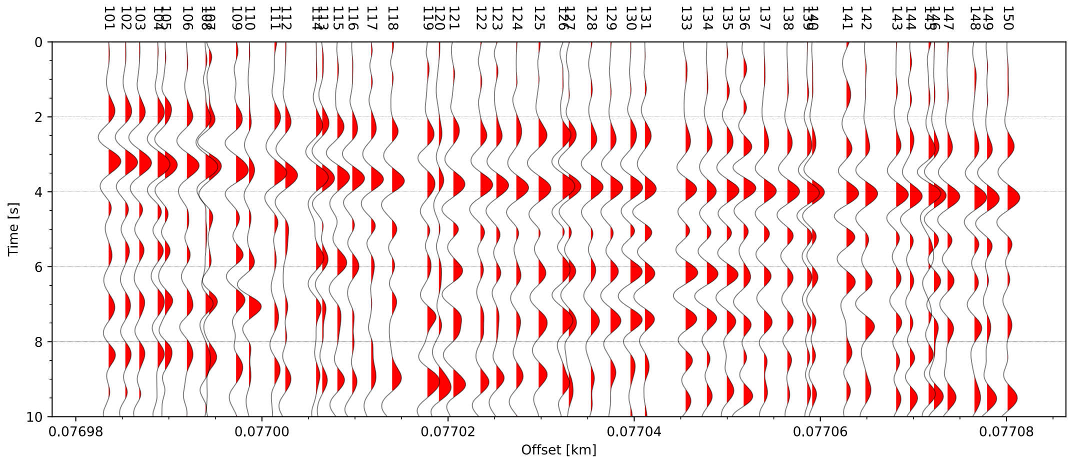


**Figure S2.** Vertical-component seismograms along Line 1 for 10/31/23 Chile M6.7 teleseismic event, filtered between 0.1–1 Hz.

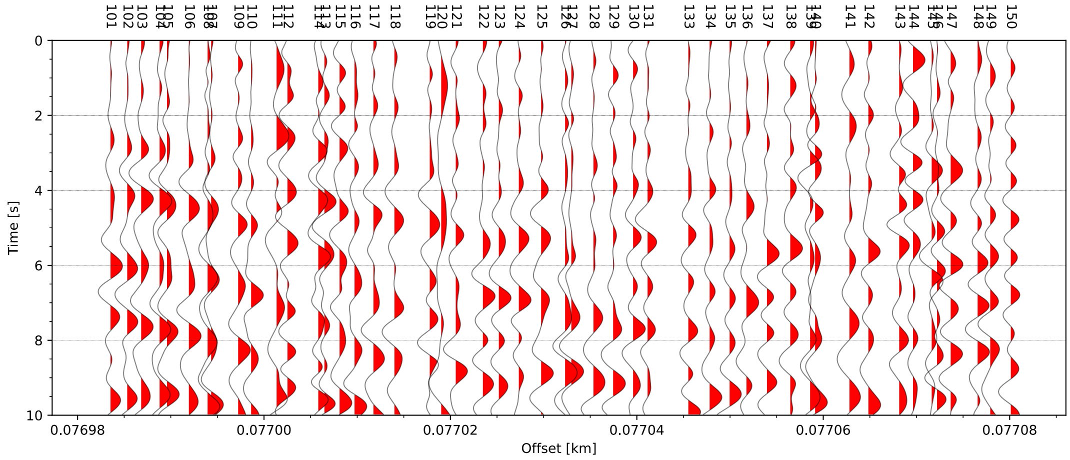

**Figure S3.** North-component seismograms along Line 1 for the 10/31/23 Chile M6.7 teleseismic event, filtered between 0.1–1 Hz.

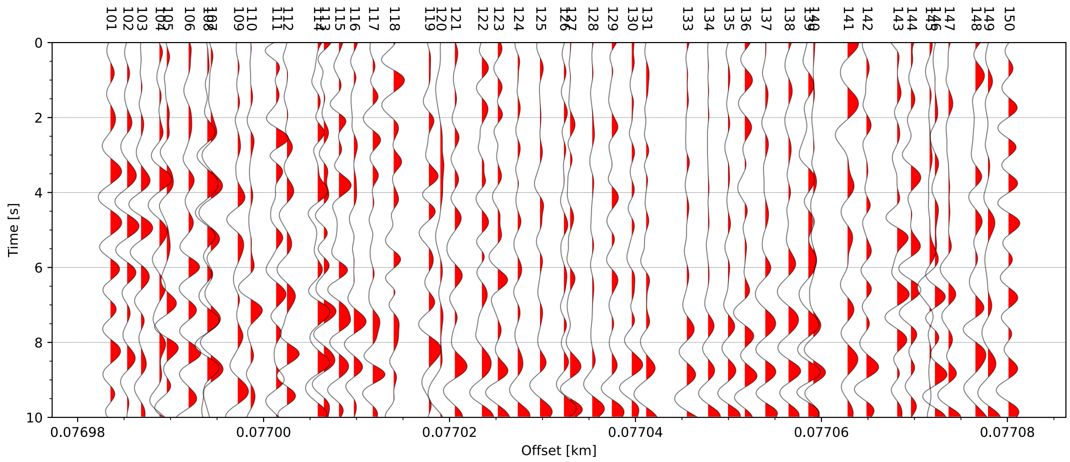


**Figure S4.** East-component seismograms along Line 1 for the 10/31/23 Chile M6.7 teleseismic event, filtered between 0.1–1 Hz.

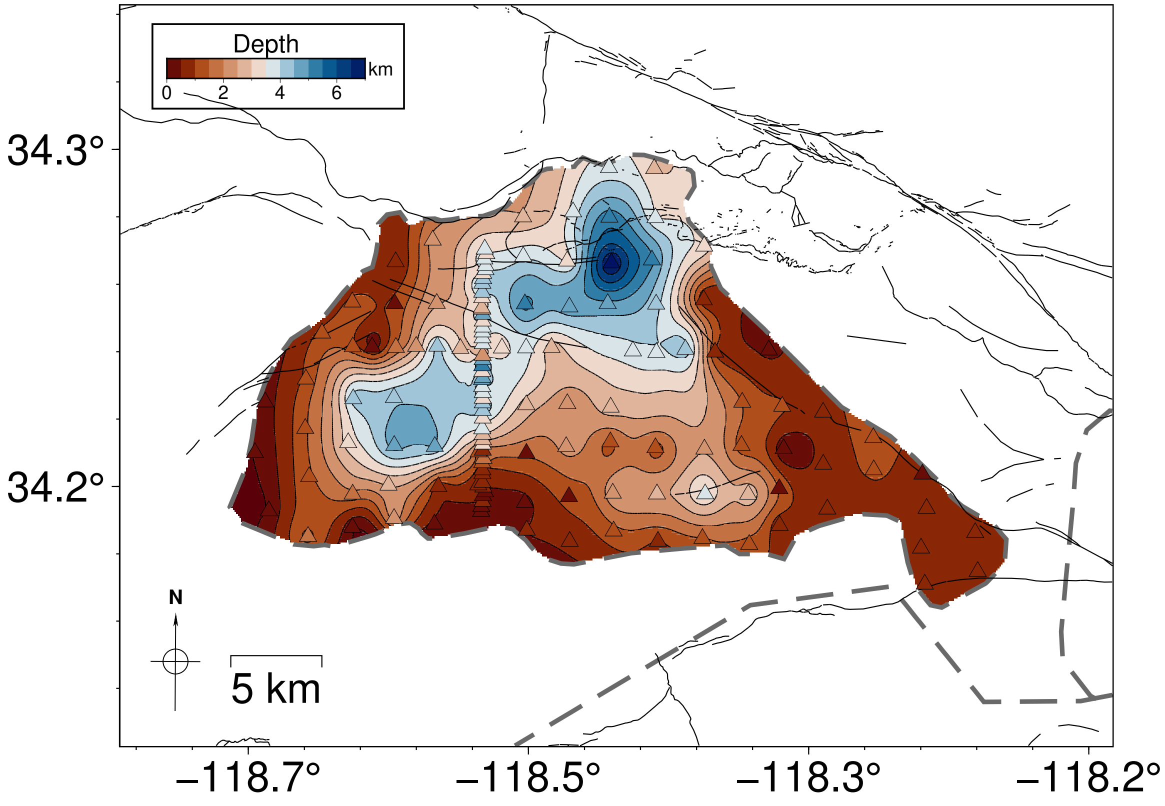


**Figure S5.** 3D Basin depth map under the baseline model. The gravity guided pick assume -50 kg/m$^3$ of apparent density contrast.

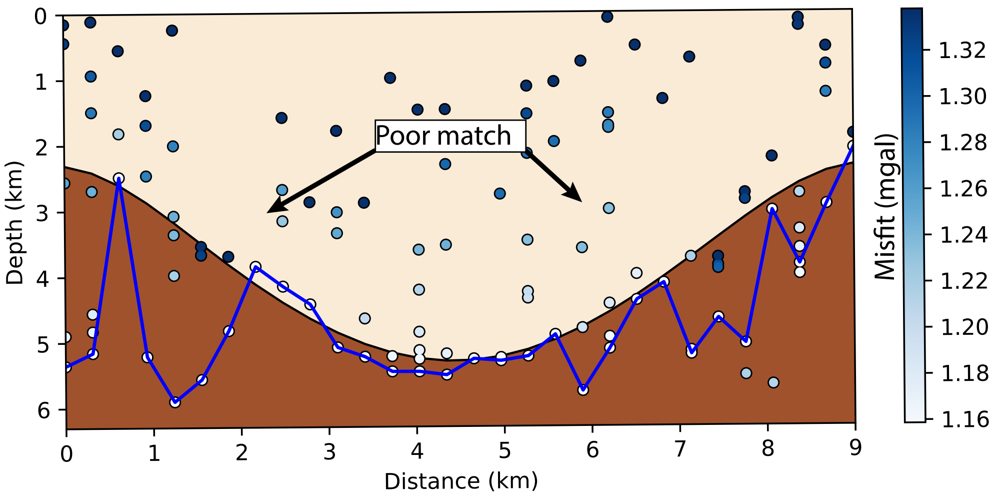


**Figure S6.** Synthetic example with constant density of -20 kg/m$^3$. The colorbar shows the misfit between the predicted Bouguer gravity and the true Bouguer gravity. The blue line highlights the lowest misfits points along the profile.

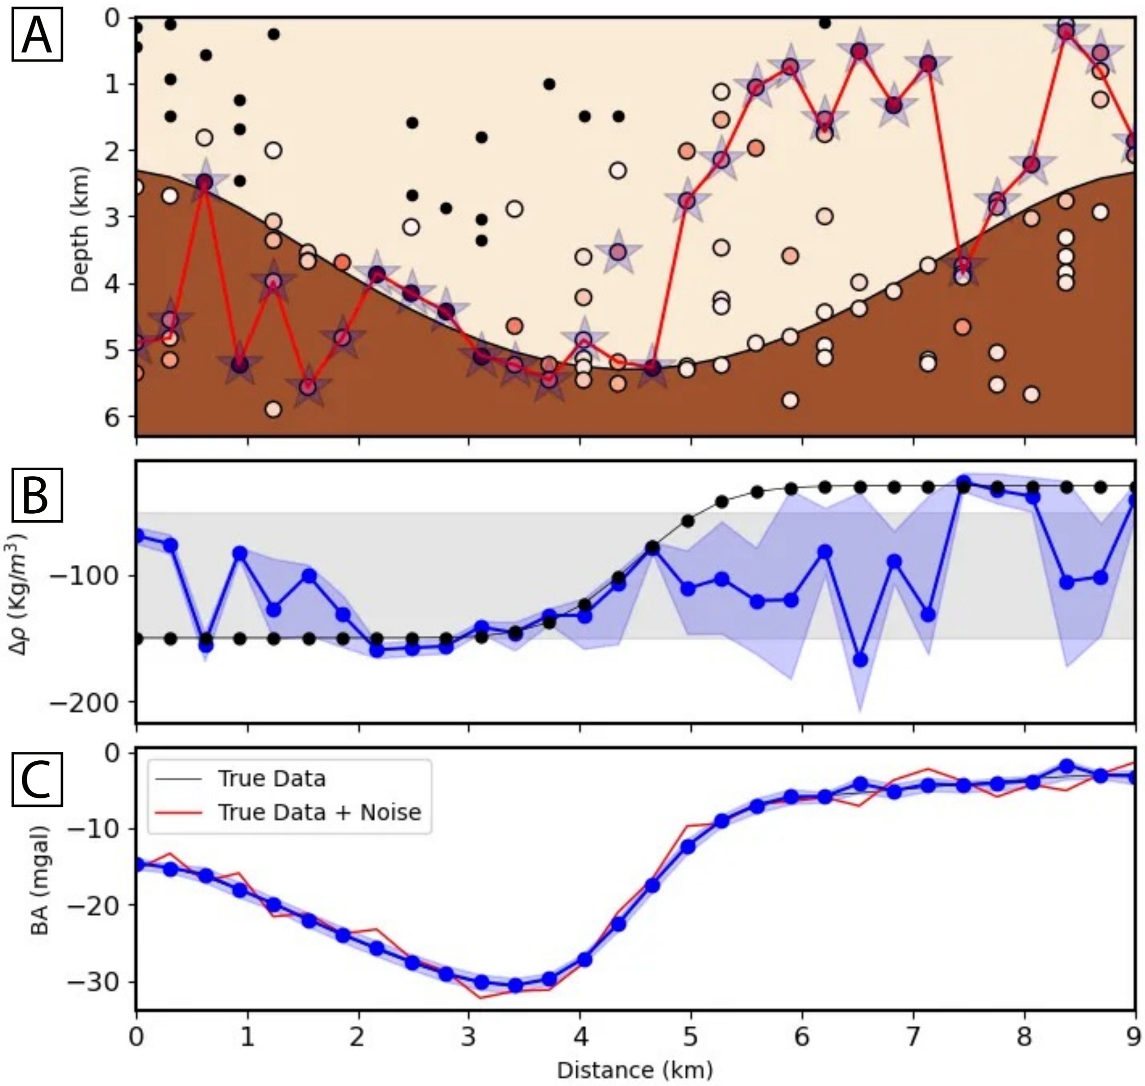


**Figure S7.** Synthetic example with no regularization. The points on panel (A) are colored by probability, as inferred from the density probability posterior. Blue stars on panel (A) indicate the median time of that probability distribution, i.e., the most likely time to basement. Panel (B) shows the density posterior along with 16th and 84th percentiles, from which other quantities are inferred. Panel (C) shows the median BA and 16th/84th percentiles.

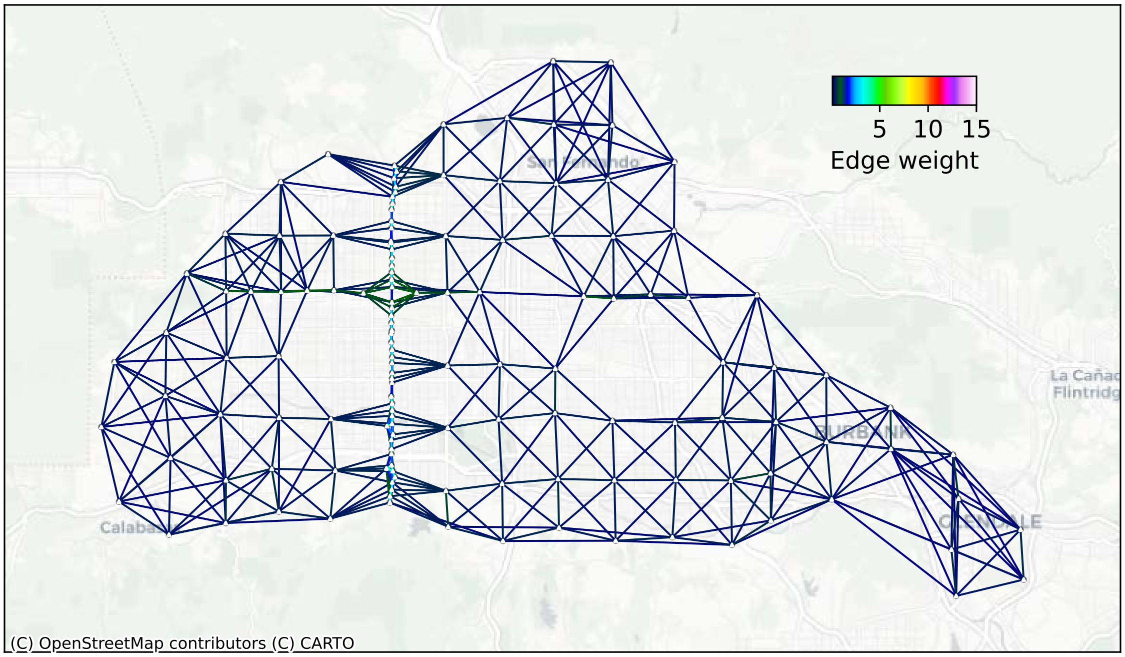


**Figure S8.** Graph Network of the 3D Bayesian inference model. The colored lines are the connections between the nodes (white triangle). The colorbar references to the weight of the connection.

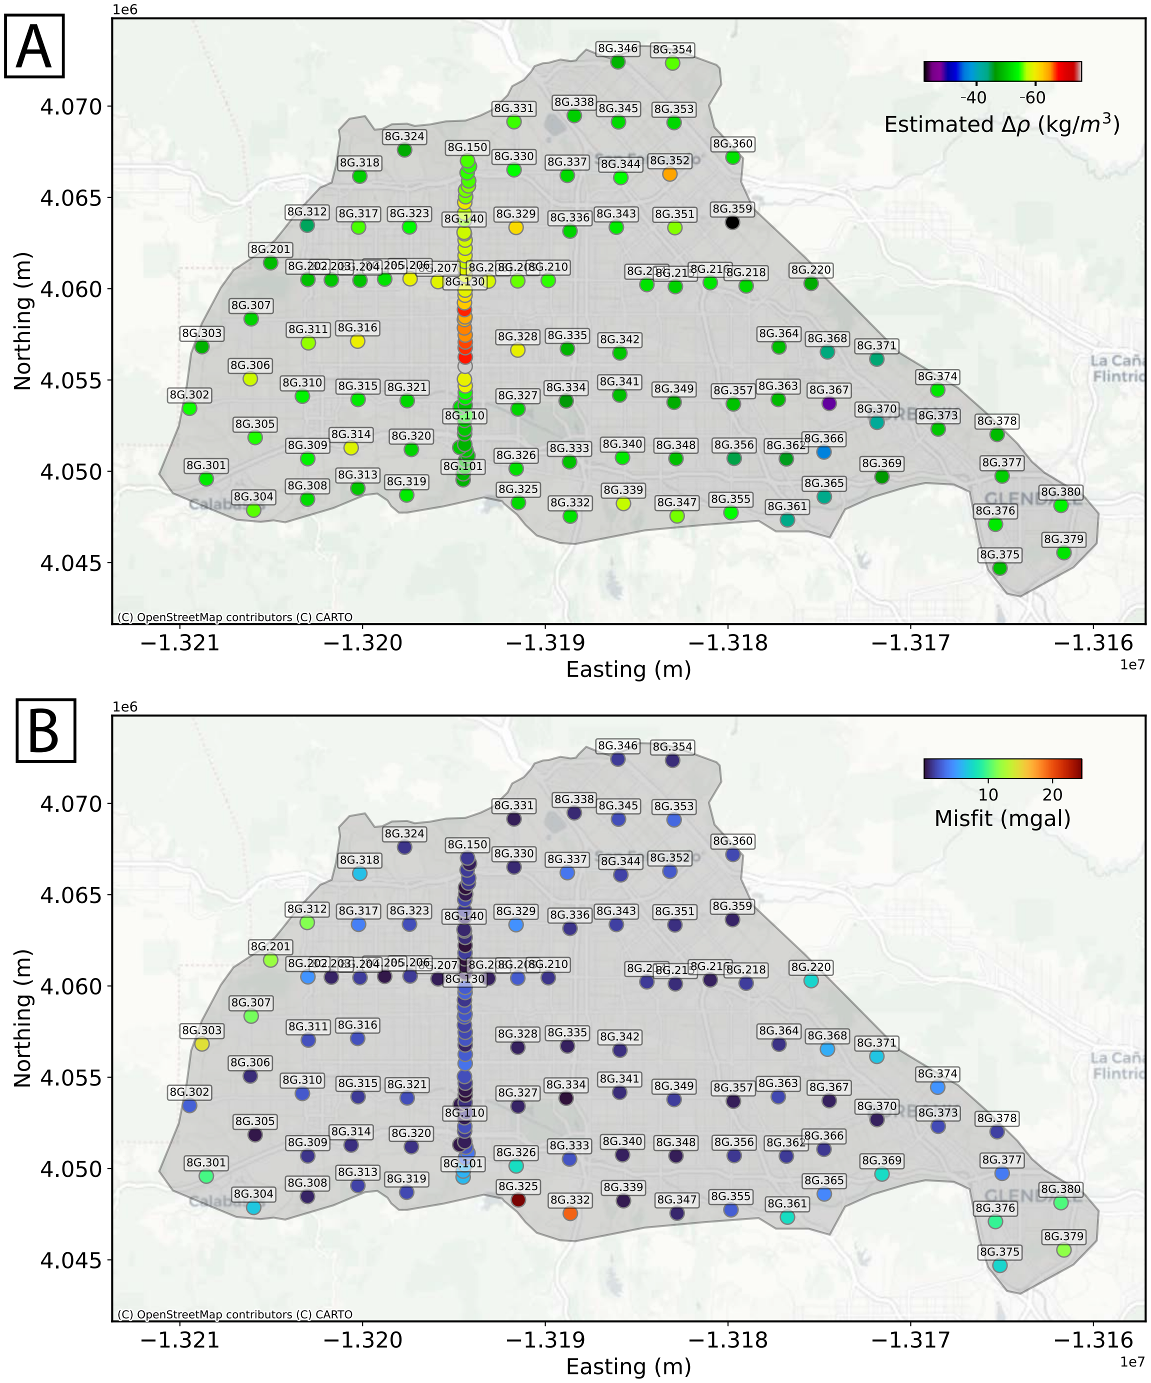


**Figure S9.** Median effective density contrast values and misfits of the BA (predicted - observed).

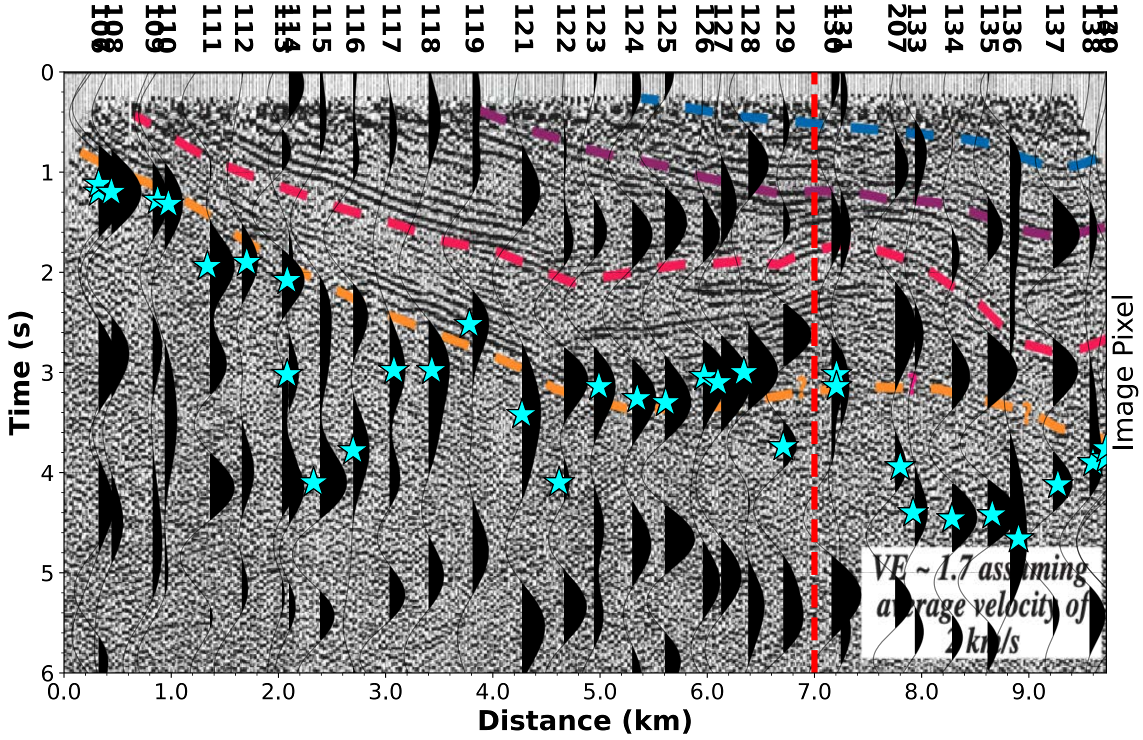


**Figure S10.** Receiver Functions overlaid on industry profile 2893-O (Langenheim et al., 2011). The stars indicate the best pick for the sediment-basement interface.

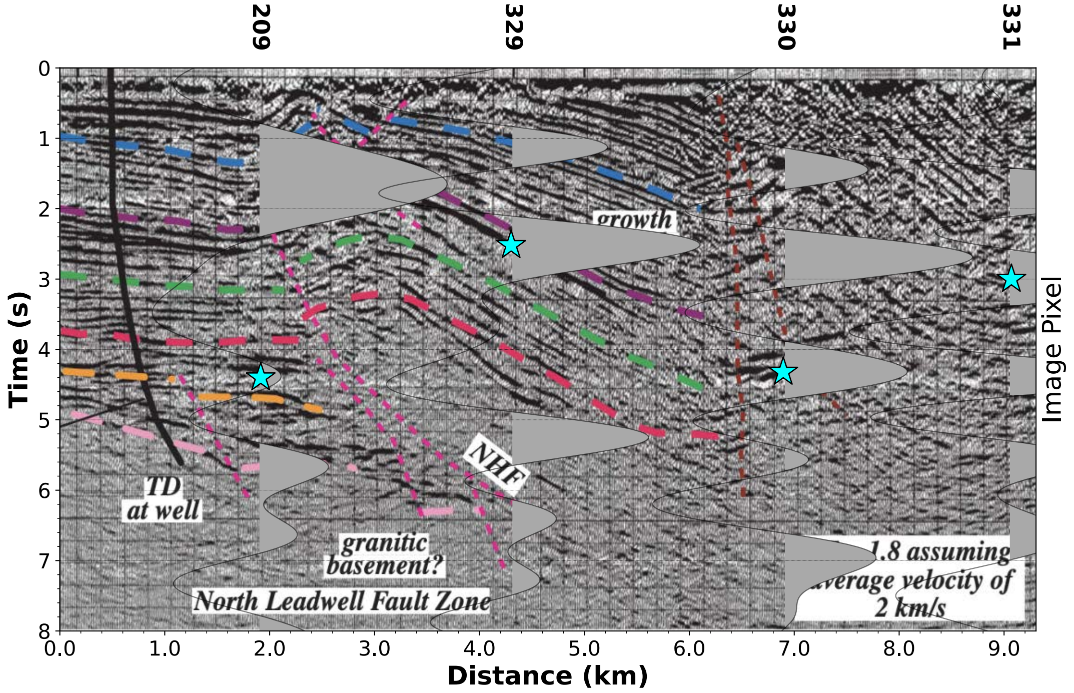


**Figure S11.** Receiver Functions overlaid on industry profile SFV-85-12 (Langenheim et al., 2011). The stars indicate the best pick for the sediment-basement interface.

| Well Number | API | Latitude | Longitude | Depth (km) |
|---|---|---|---|---|
| 1 | 403705201 | 34.288403 | -118.38118 | 1.63 |
| 2 | 403721802 | 34.257713 | -118.454887 | 3.12 |
| 3 | 403705634 | 34.179424 | -118.659691 | 0.94 |
| 4 | 403705974 | 34.203827 | -118.447884 | 1.54 |
| 5 | 403705969 | 34.175121 | -118.425677 | 1.15 |

**Table S1.** Boreholes that reach basement in the San Fernando Valley.

References From the Supporting Information

Clayton, R. (2022, August). *Gravity Data For Southern California*. CaltechDATA. https://doi.org/10.22002/D1.20256

Langenheim, V. E., Wright, T. L., Okaya, D. A., Yeats, R. S., Fuis, G. S., Thygesen, K., & Thybo, H. (2011). Structure of the San Fernando Valley region, California: Implications for seismic hazard and tectonic history. *Geosphere*, *7*(2), 528–572. https://doi.org/10.1130/GES00597.1
